# Supplementary material for: Contact2Grasp: 3D Grasp Synthesis via Hand-Object Contact Constraint
Source: arXiv:2210.09245 source file (2023-05-06)
Supplement: Supplementary file 1 [file appendix.tex]

\section{Appendix}

\begin{figure*}[htbp]
  \centering
    \includegraphics[width=\textwidth]{fig/qualitative2_ho3d.pdf}
  \caption{Generated contacts and grasps on out-of-domain HO-3D objects. We generate 2 grasps for each object. For each result, we visualize both the generated contact map (right) and the corresponding grasping pose (left).}
  \label{fig.qualitative result}
%   \vspace{-0.1cm}
\end{figure*}

\subsection{Evaluation on the HO-3D Dataset}

\textbf{HO-3D}  We further validate our framework on the HO3D dataset~\cite{hampali2020honnotate}, which is a real-world datset and includes 10 objects. Due to the limitation of number of objects and grasp types, we follow the work~\cite{karunratanakul2020grasping} and use the dataset for testing the models trained on Obman. Examples of generated grasps of our method are shown in Figure \ref{table:ho3d}. 

% \textbf{Local Refinement Details} For the inference refinement on the HO3D, we adopt Adam optimizer with a learning rate of $1.00\times 10^{-4}$  to update the GraspNet decoder (MLP) parameters. The number of steps is 150.

% It should be mentioned that we fix the GraspNet encoder (PointNet) paramenters and only update the parameters of decoder (MLP) during the refining process. The above strategy is implemented on all datasets.

Table \ref{table:ho3d} compares the quality of generated grasps of our method to that of the baselines and existing works on HO3D. Our method improves the Param2Mesh baseline on the penetration metrics and the contact ratio significantly. 
It outperforms the state-of-the arts on all metrics except the penetration volume. Specifically our method achieves the best performance on simulation displacement (2.72 $cm$), contact rate (99.11$\%$) and grasp success rate (47.11$\%$) metrics. 

Notice that the contact ratio of all methods in  Table \ref{table:ho3d} is not so good as that of testing results on Obman in the main paper, which mainly results from the object size difference of these two datasets. The method proposed in~\cite{jiang2021hand} has difficulty in generalizing to HO3D  while our method adapts to the new objects of larger size better regarding the contact ratio metric.

\begin{table*}[h]
    \centering
    % \scriptsize
    \begin{tabular}{lcccccc}
        \toprule
        \multirow{2}*{\textbf{Methods}} & \multicolumn{2}{c}{\textbf{Penetration, $\downarrow$}}  &\multicolumn{2}{c}{\textbf{Simulation, $\downarrow$}} &\multirow{2}*{\textbf{CR($\uparrow$)}}
        &\multirow{2}*{\textbf{Sim$_{SR}$($\uparrow$)}}\\
        \cmidrule(r){2-3} \cmidrule(r){4-5}
        &\textbf{Dep} &\textbf{Vol} &\textbf{Mean} &\textbf{Var}\\
        \midrule
        GraspField &1.46 &14.90 &3.45 &$\pm$3.92 &90.10 &- \\
        GraspTTA &1.09 &4.88 &3.80 &$\pm$4.20 &92.31 &24.75 \\
        Ours &\textbf{0.71} &\textbf{4.00} &\textbf{2.72} &\textbf{$\pm$2.78} &\textbf{99.11}  &\textbf{47.11}\\
        \midrule
        GT  &2.94 &6.08 &4.31 &$\pm$4.42 &91.60 &26.07  \\
        % \midrule
        % Ours w/o refine (GT) &0.43 &4.68 &1.97 &$\pm$2.40 &100.00 \\
        % Ours (GT) &0.36 &3.75 &1.98 &$\pm$2.46 &99.96 \\             
        \bottomrule
    \end{tabular}
        \caption{Quantitative Comparison on HO3D dataset}
    \label{table:ho3d}
\end{table*}

\subsection{More Visualization on the ContactPose Dataset}
In Figure~\ref{fig.qualitative result2}, we present the generated results on objects from the ContactPose~\cite{brahmbhatt2020contactpose} training group. We can observe that the some generated contacts and predicted grasps are corresponding with the object affordance.

\begin{figure*}[htbp]
  \centering
    \includegraphics[width=\textwidth]{fig/qualitative_contactpose.pdf}
  \caption{Generated contacts and grasps on ContactPose objects from the training group.We select 12 out of 21 objects for the visualization. For each object, we visualize both the generated contact map (right) and the corresponding grasping pose (left). Note that the generated grasps is more realistic and reasonable.}
  \label{fig.qualitative result2}
%   \vspace{-0.1cm}
\end{figure*}

\subsection{The mathematical descriptions of metrics}
\textbf{Simulation Displacement.} We choose this metric by following~\cite{hasson2019learning} as it provides a way to measure the physical realism of generated grasps and we can compare with~\cite{jiang2021hand,taheri2020grab} on this metric. The simulation environment (PyBullet physics engine) checks the force closure. If the force closure is not met, objects fall and cause the displacement of objects after placing generated grasps. Therefore, the displacement metric actually has the force-closure metric included. The displacement is defined as $Dist =f(x,x')$ if $f(x,x')<0.1$, else $Dist =0.1$, where $f(x,x') =\Vert x- x' \Vert_2$. $x, x'$ represent the initial and end position of object center.

\textbf{Penetration volume ($P_v$) and depth ($P_d$)} follows the definition in~\cite{hasson2019learning},To calculate the penetration, we first voxelize a grasp and an object, then a sign distance field (SDF) is constructed for the object (positve inside the object and negative outside). For each voxel of the grasp, if its value in the object SDF is positive, it is an intersected voxel.$P_v =\mu \sum_{i=0}^N v_i,  v_i \in V$, where $V$ denotes the intersection voxel set between the grasp and the object, $v_i$ represents the i-th voxel.$\mu$ denote unit size of voxel and N denotes the number of voxels. The penetration depth is the maximum distance of the penetration, defined as$P_d = \underset{v_i\in V}{max}SDF(v_i)$, where $SDF(v_i)$ denotes the distance value of an intersected voxel.

\textbf{Contact Rate (CR).} We define a contact between the object and the hand when any point on the surface of the hand is on or inside the surface of the object~\cite{karunratanakul2020grasping}.The formuation is defined as:
\begin{equation}
    \small
    C_r =\frac{1}{N_s}\sum_{i=0}^{N_s}x_i,  
\end{equation}
\begin{equation}
    \small
        x_i =\begin{cases}1, \quad (max(C'')\neq 0) \wedge (P_v>0)  \\  0, \quad else \end{cases},
\end{equation}
where $N_s$ denotes the number of generated samples.$x_i$ denotes the i-th sample.

\textbf{Grasp Success Rate (Sim$_{SR}$)} is a comprehensive metrics. It define a  grasp with both less penetration and simulation displacement as positive sample.  The definition of Sim-SR is:
\begin{equation}
    \small
    Sim_{SR} =\frac{1}{N_s}\sum_{i=0}^{N_s}x_i,
\end{equation}
\begin{equation}
    \small
    x_i =\begin{cases}1, \quad (P_v<\eta) \wedge (Dist<\alpha)  \\  0, \quad else \end{cases},
\end{equation}
where $\eta=5 (cm^3)$ and $\alpha=2.0 (cm)$ denote threshold of penetration volume and simulation displacement respectively.

\textbf{Diversity (Div)} is proposed to measure the diversity of generated result. The definition is:
\begin{equation}
    \small
            Div =\frac{1}{N_g(N_g-1)}\sum_{i=0}^{N_g}\sum_{k=0}^{N_g}\Vert v_i - v_k\Vert_2,  (i\neq k), 
    \label{eq:diversity}
\end{equation}
where $N_g$ is the number of generated samples. $v_i$,$v_k$ represent the i-th and k-th generated sample.

\subsection{The extension of our work to robotics applications}
The highlight of our work is that using generated contact map to get a reasonable grasp pose, which can be easily extended to robotics applications. In~\cite{mandikal2021learning}, the contact maps are used for input of reinforcement learning (RL) for grasping and defining better rewards. In~\cite{mandikal2022dexvip},the human poses reconstructed from videos are retargeted to the robotic hands by simply keeping the joint rotations (or keeping the task vector space) of the generated grasps. The resulting robotic hand poses are used as rewards for RL for refinement.

Based on these works, we can extend our work to robotic grasping as the following steps: (1) Retargeting human poses to posed for robotic hands. (2) Using the generated contact maps as the input for defining more detailed hand object features and better rewards for exploration under the reinforcement learning framework. (3) Using the retargeted robotic hand poses for rewards and more efficient sampling of reinforcement learning.
